# Supplementary material for: Frequency Domain-Based Diffusion Model for Unpaired Image Dehazing
Source: arXiv:2507.01275 source file (2025-07-02)
Supplement: Supplementary file 1 [file supp2.pdf]

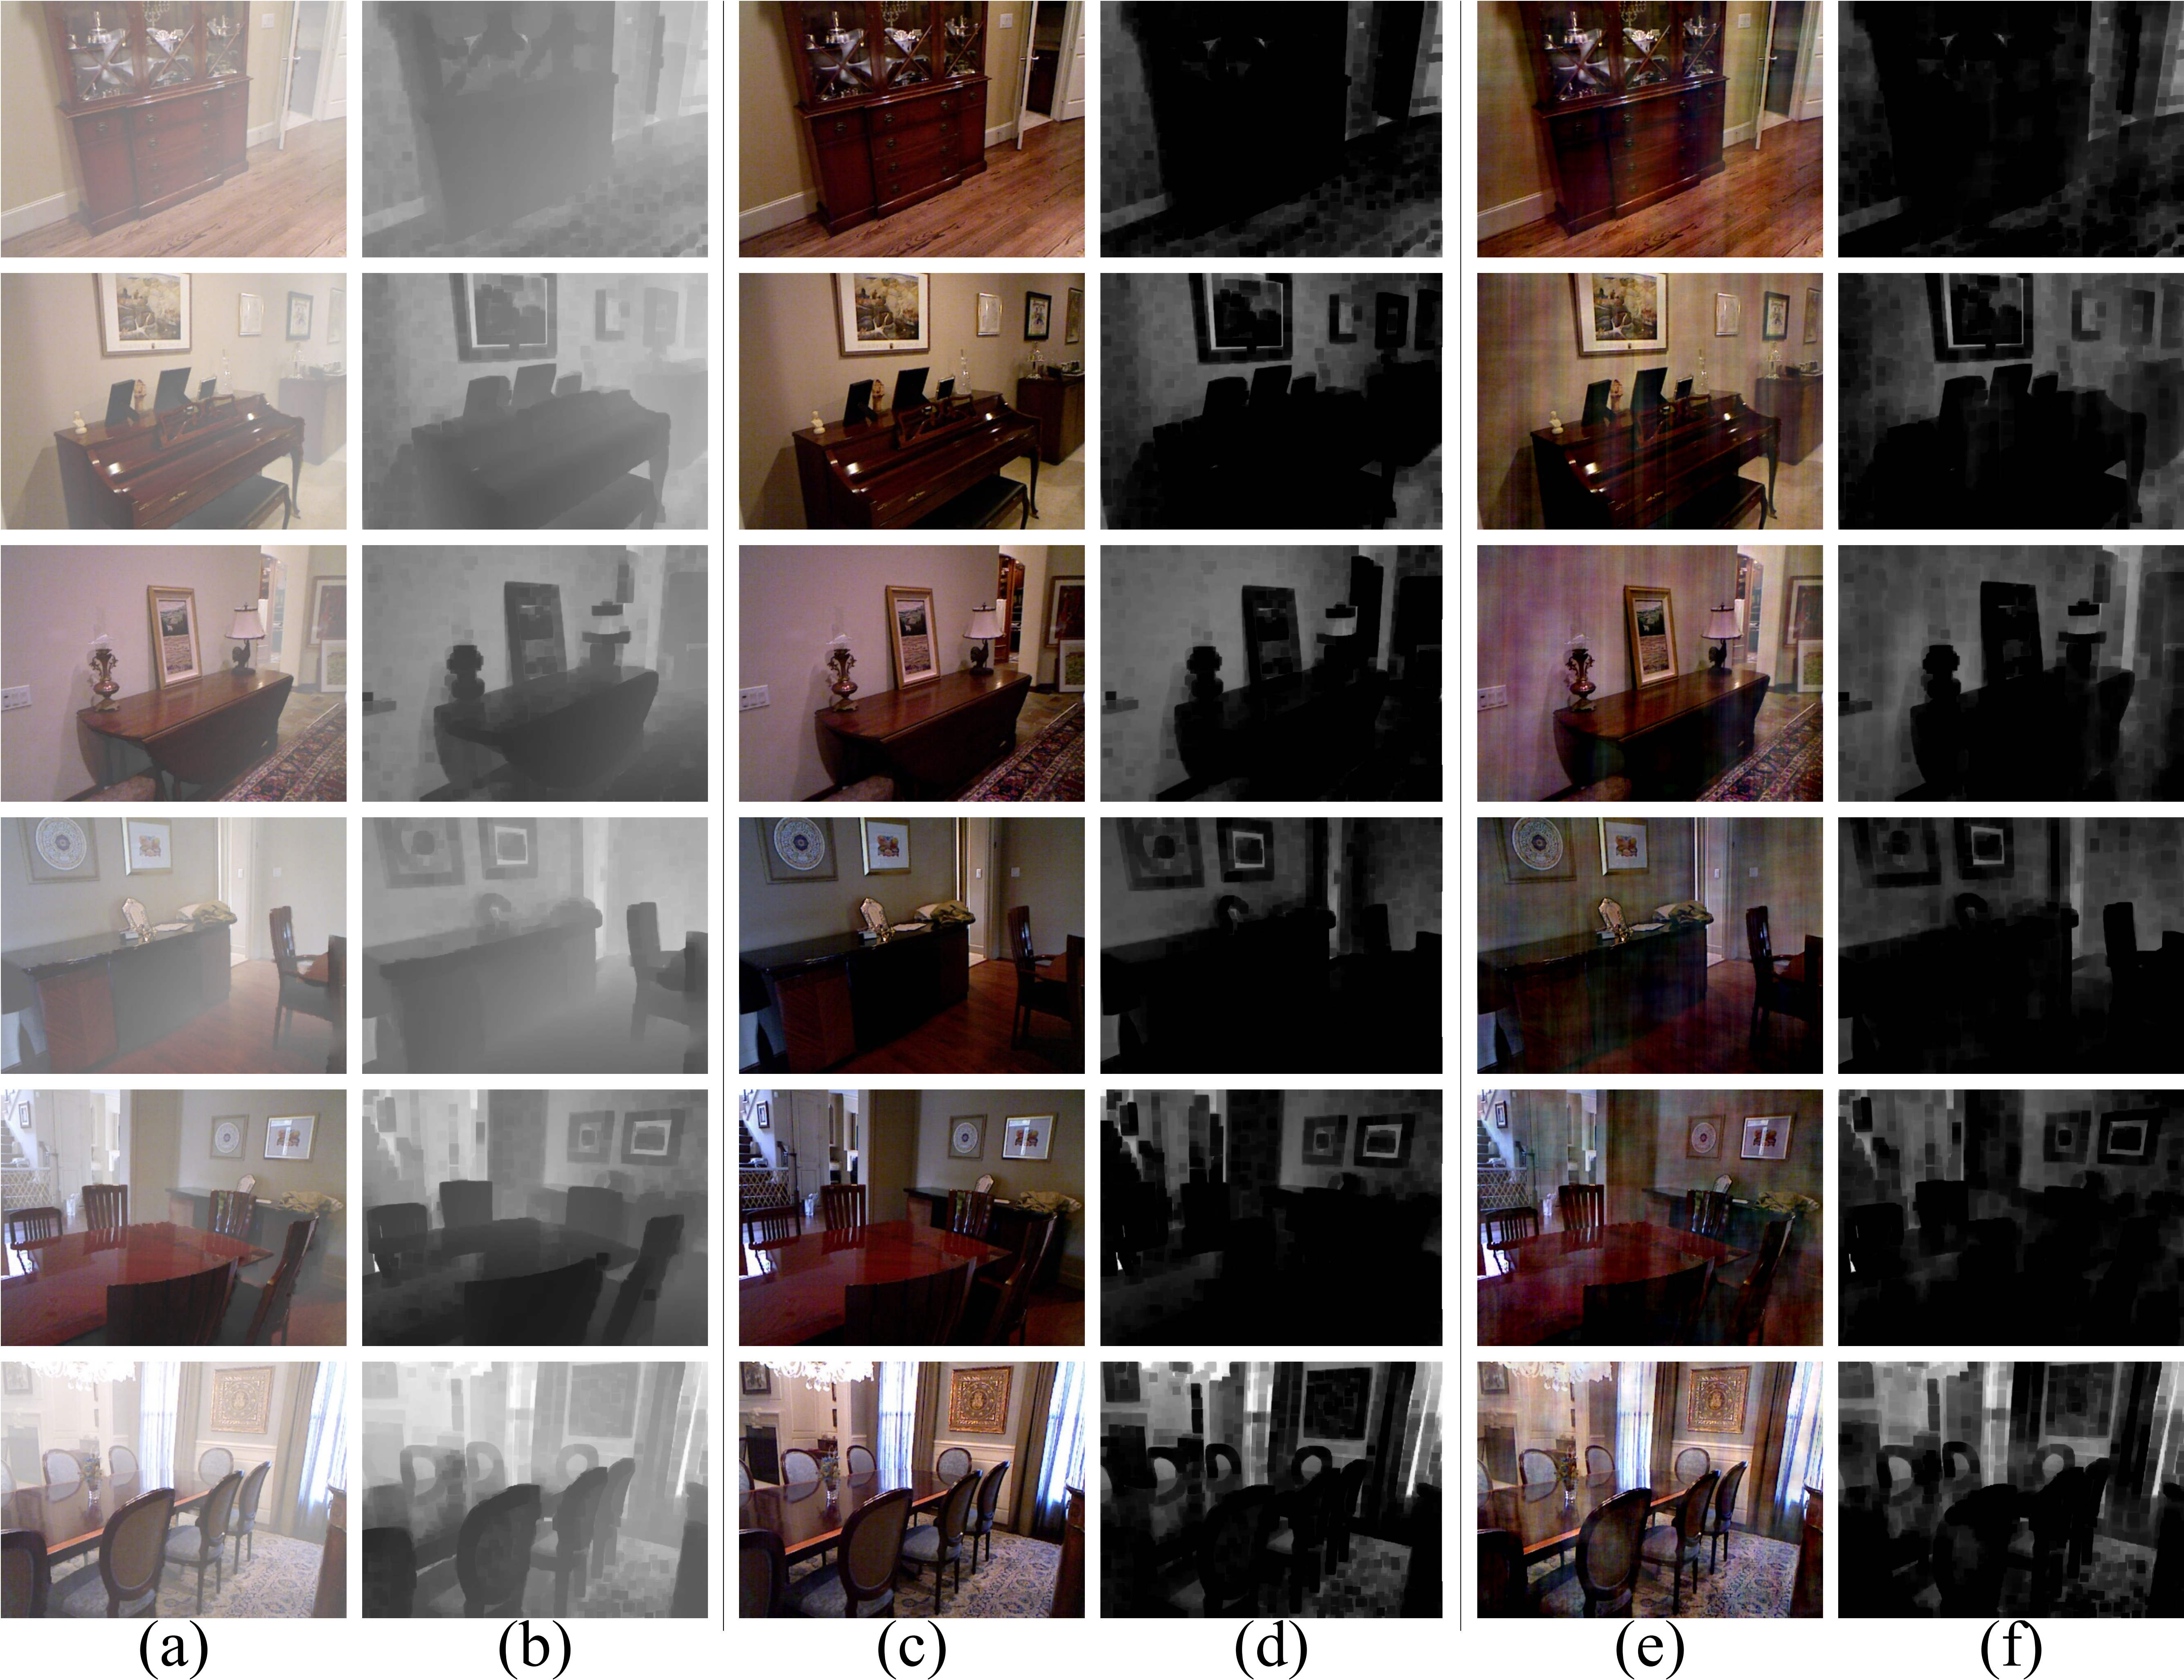

(a)

(b)

(c)

(d)

(e)

(f)



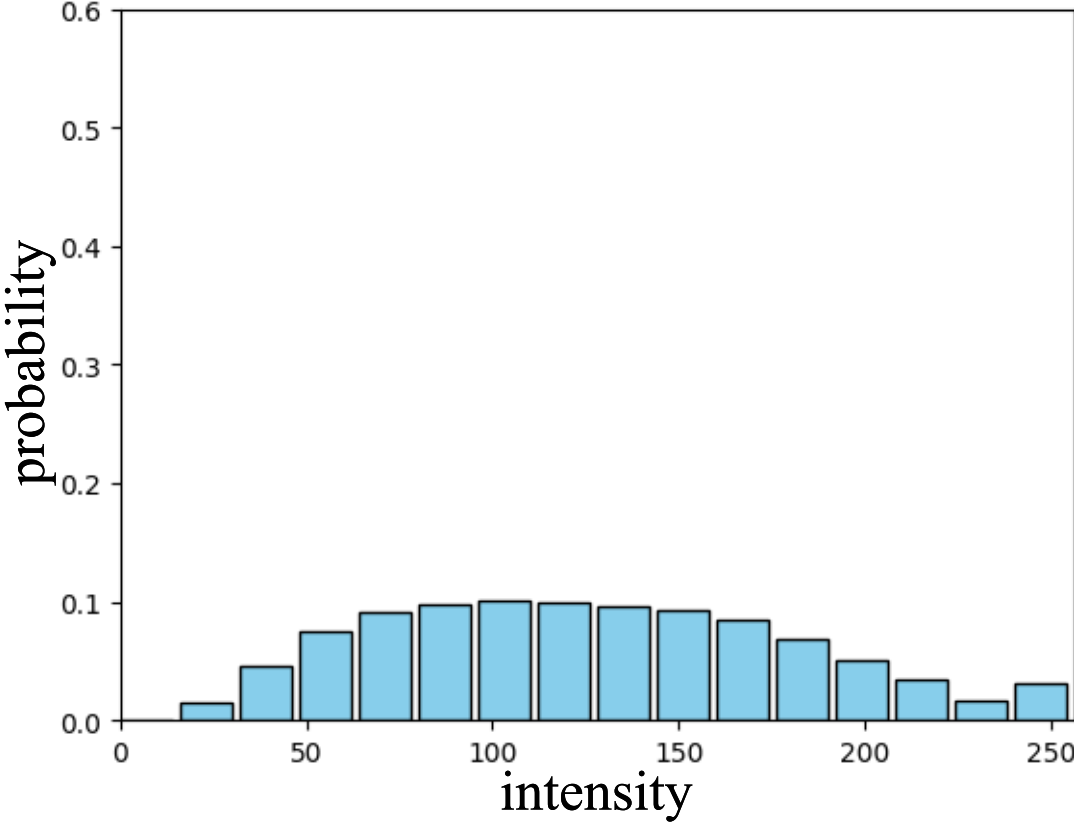

(a)

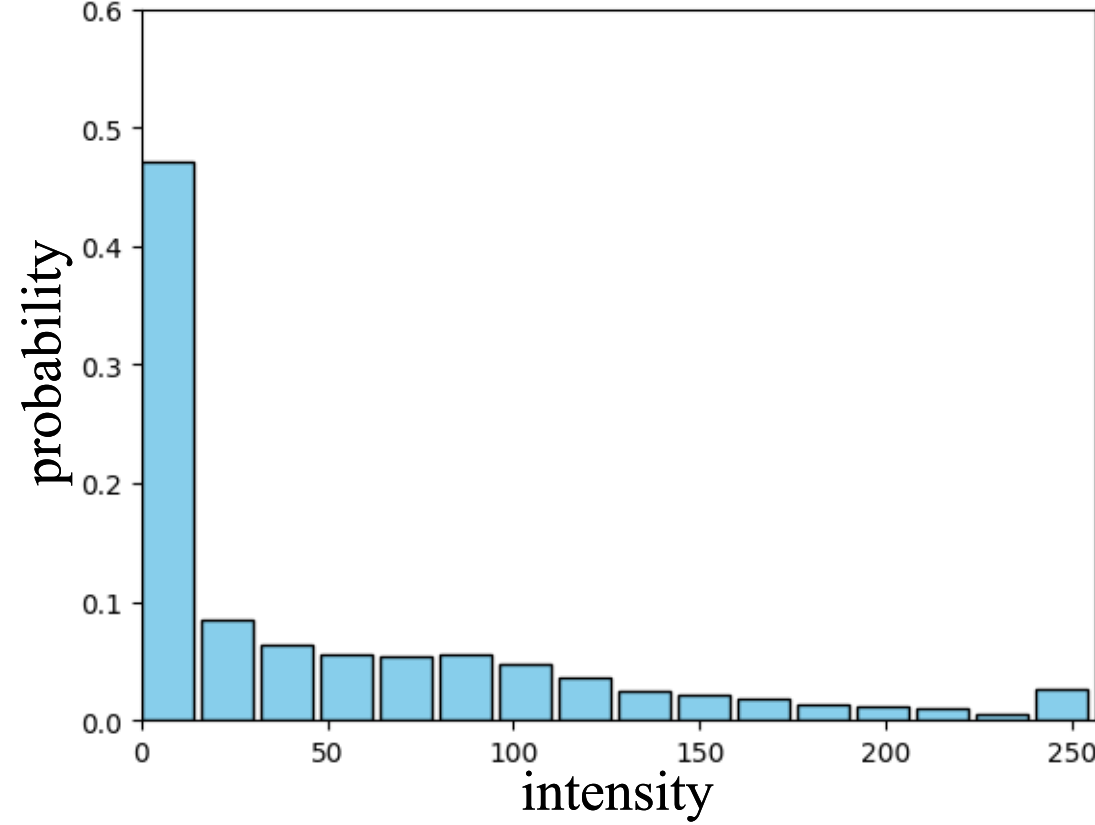

(b)

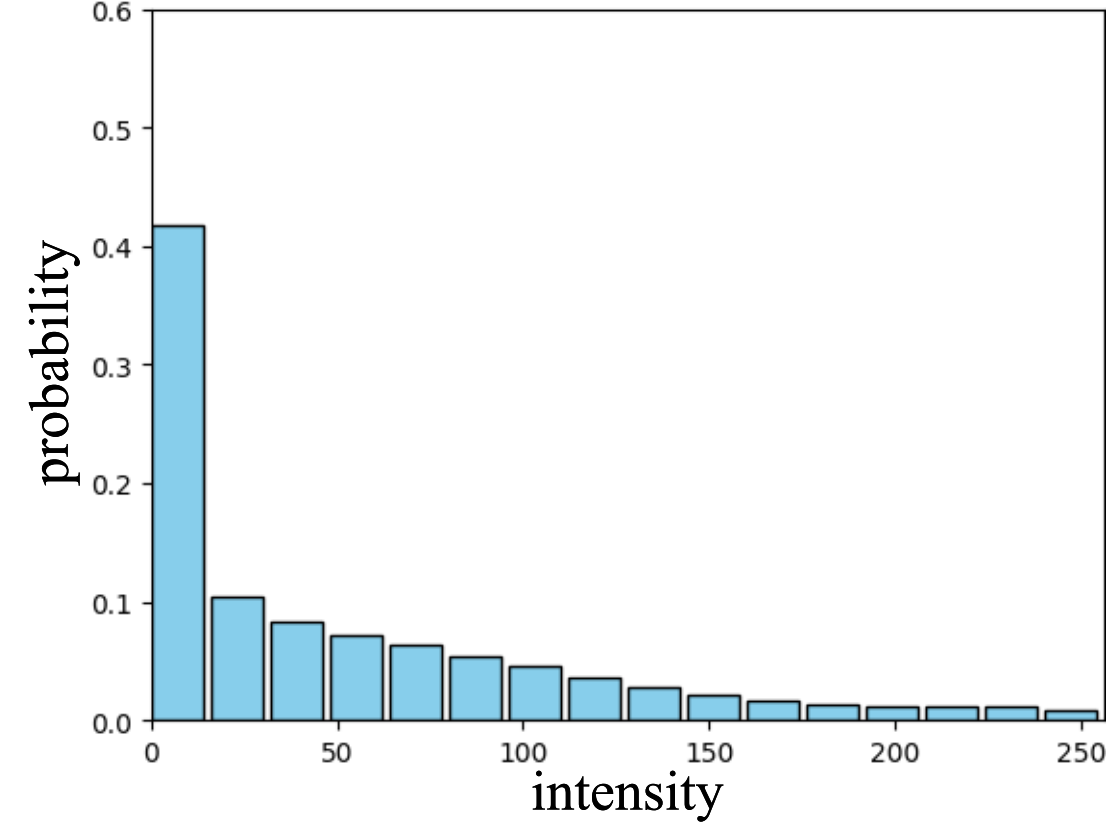

(c)

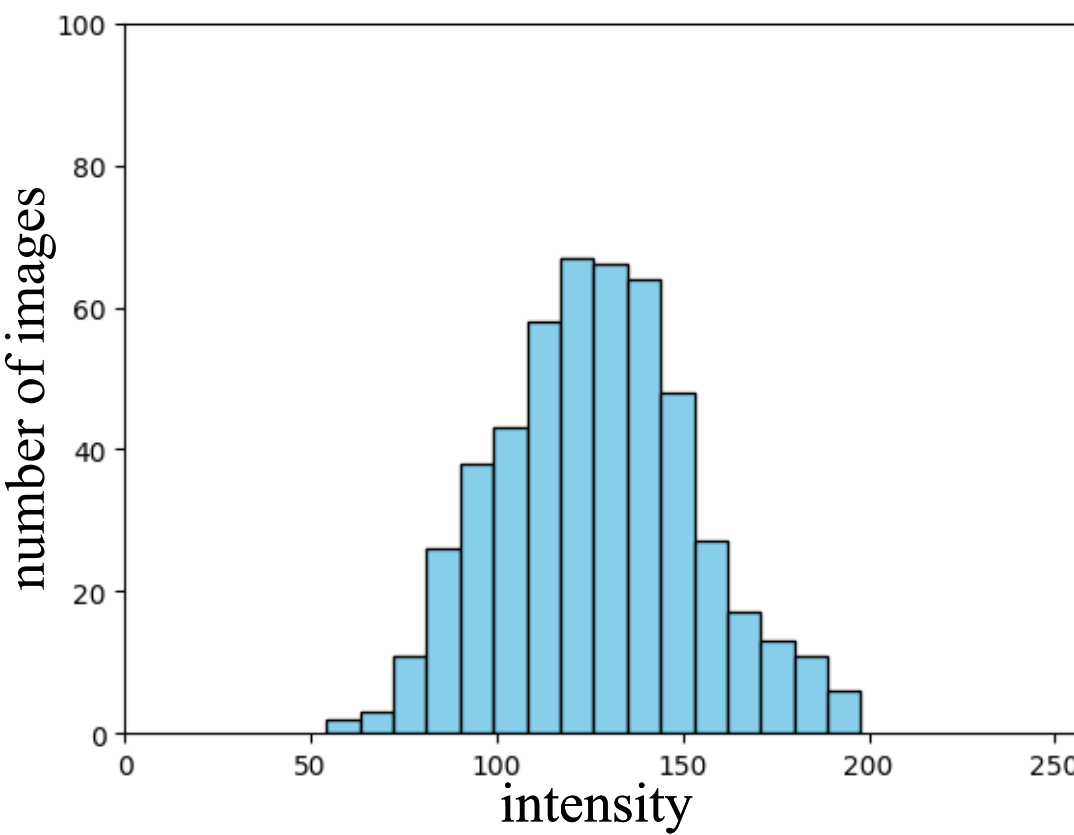

(d)

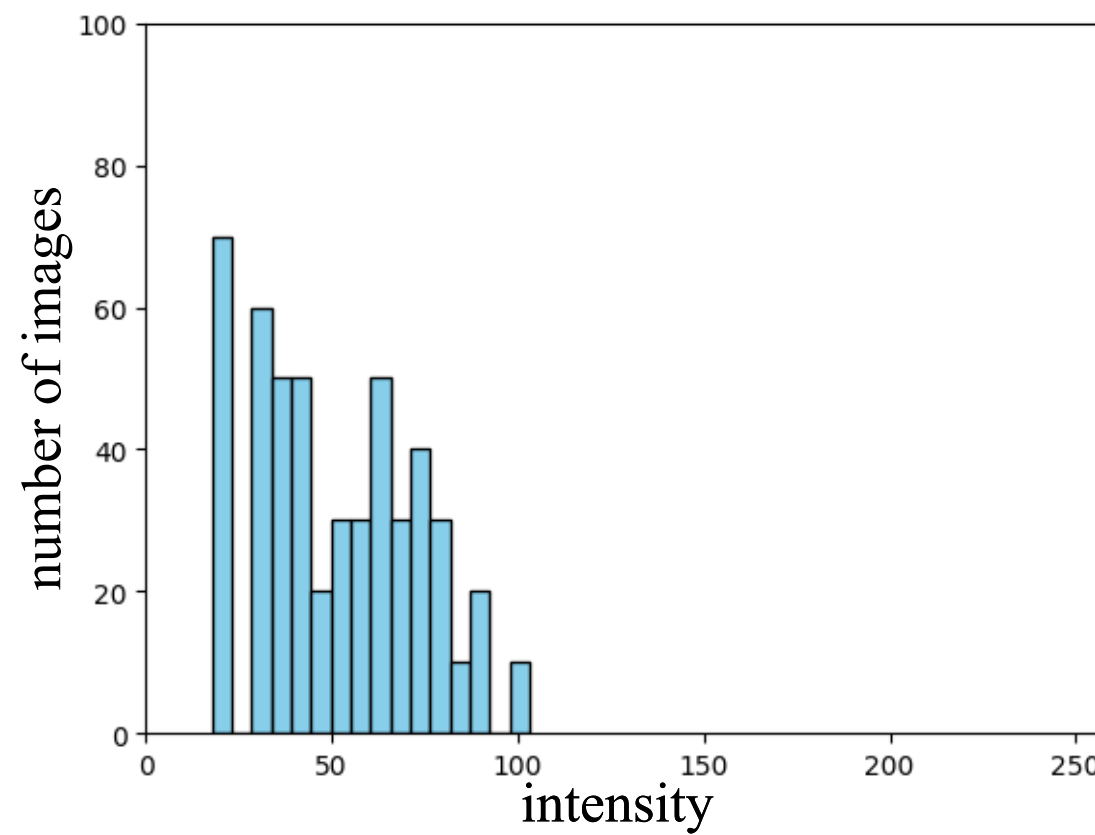

(e)

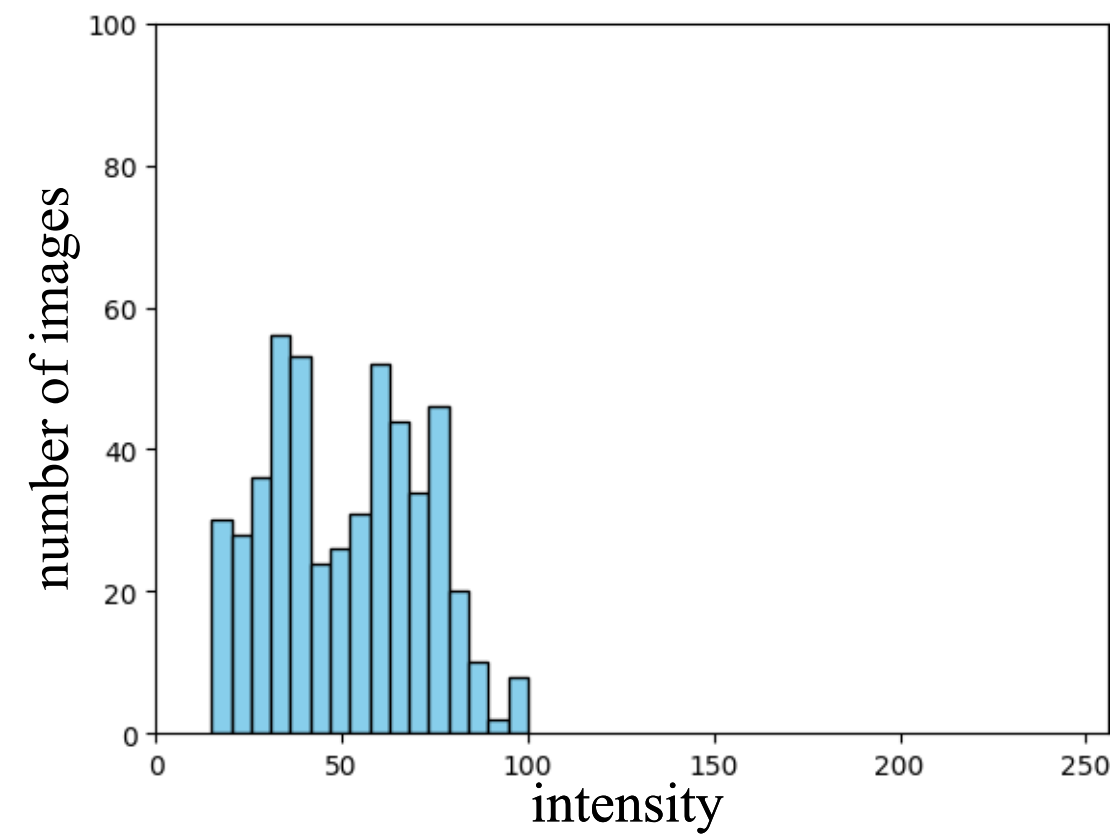

(f)

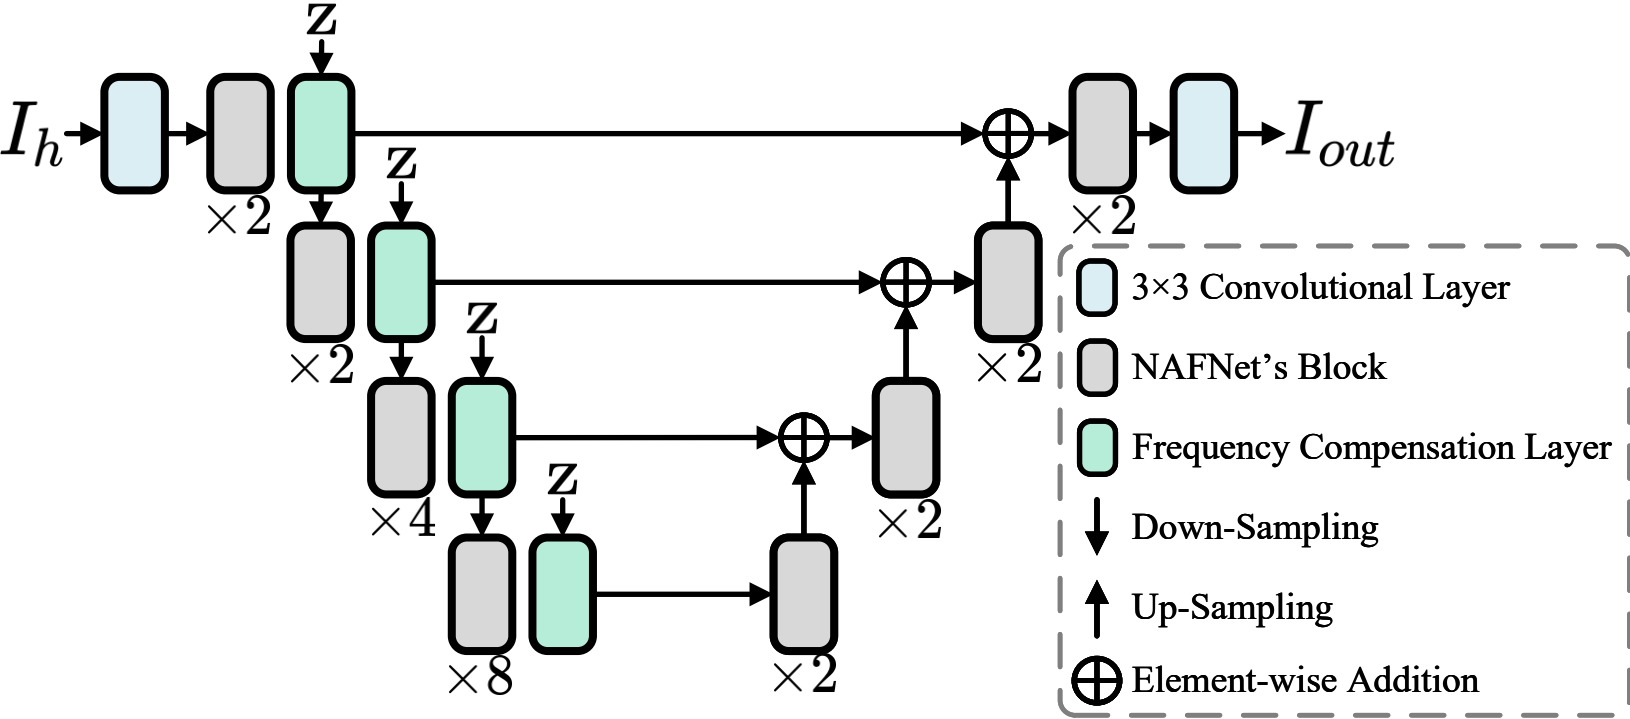



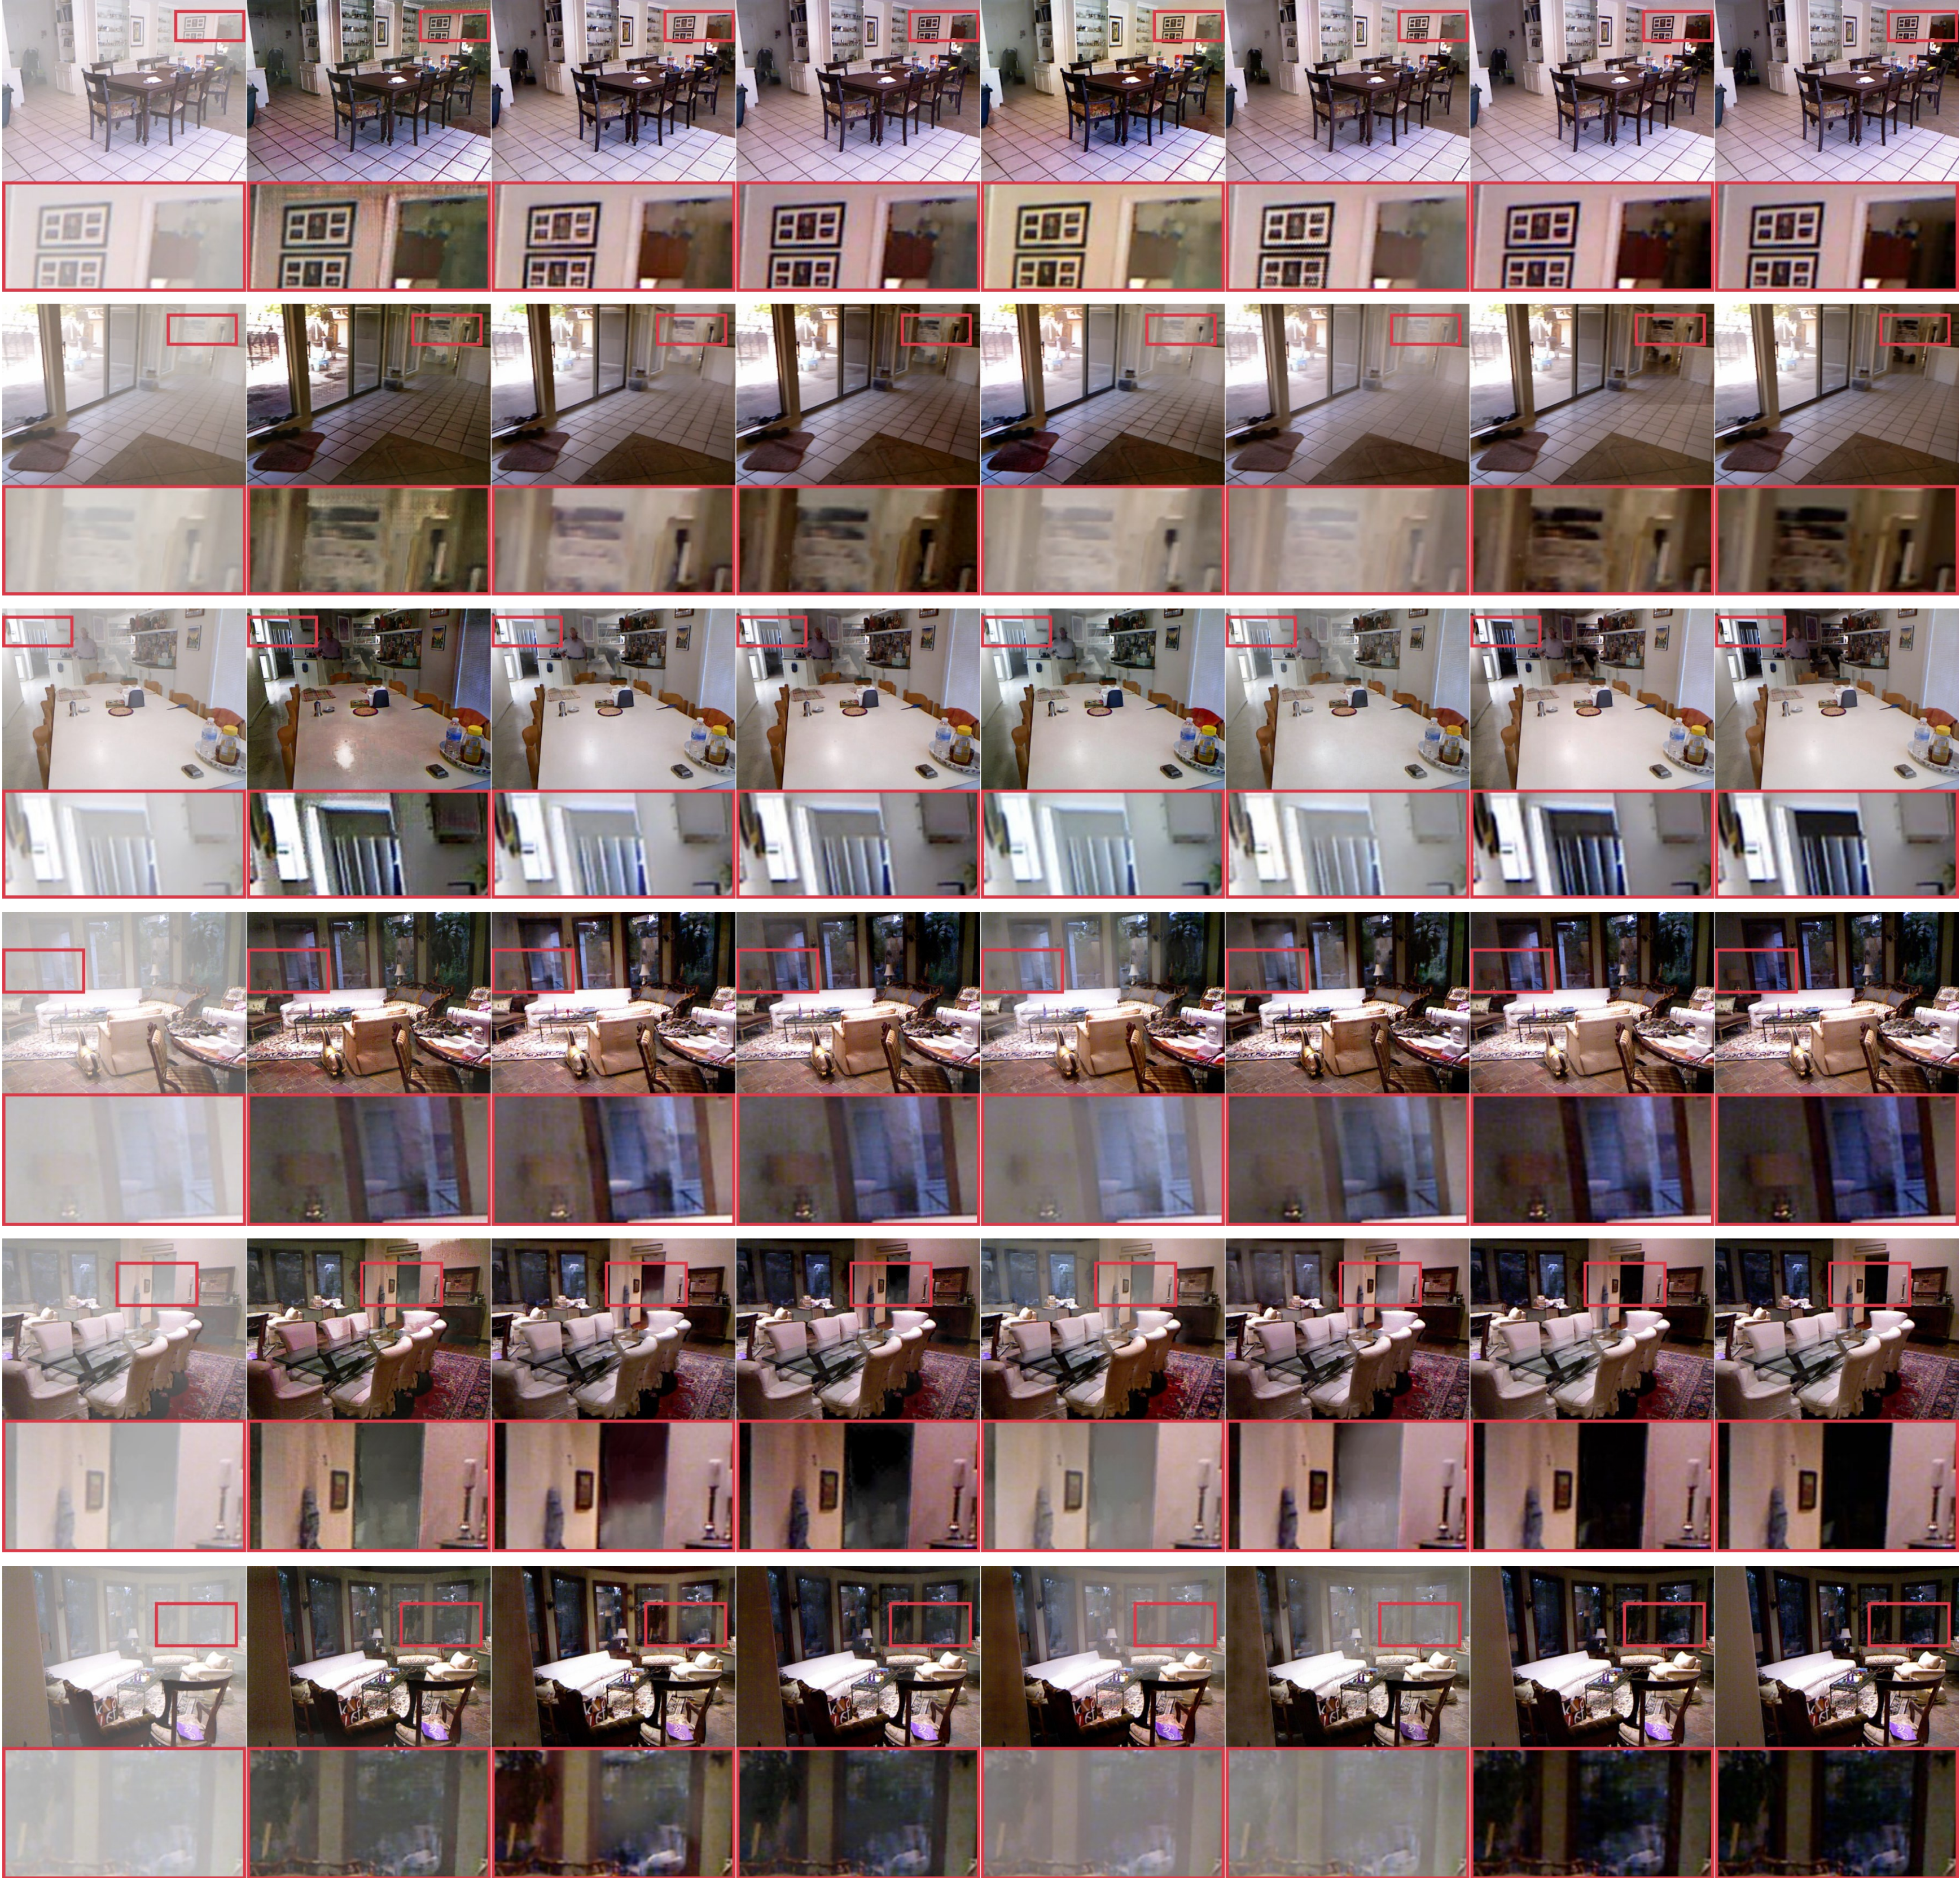

Hazy

RefinedDNet

CDD-GAN

D4

UCL-Dehaze

ODCR

Ours

GT



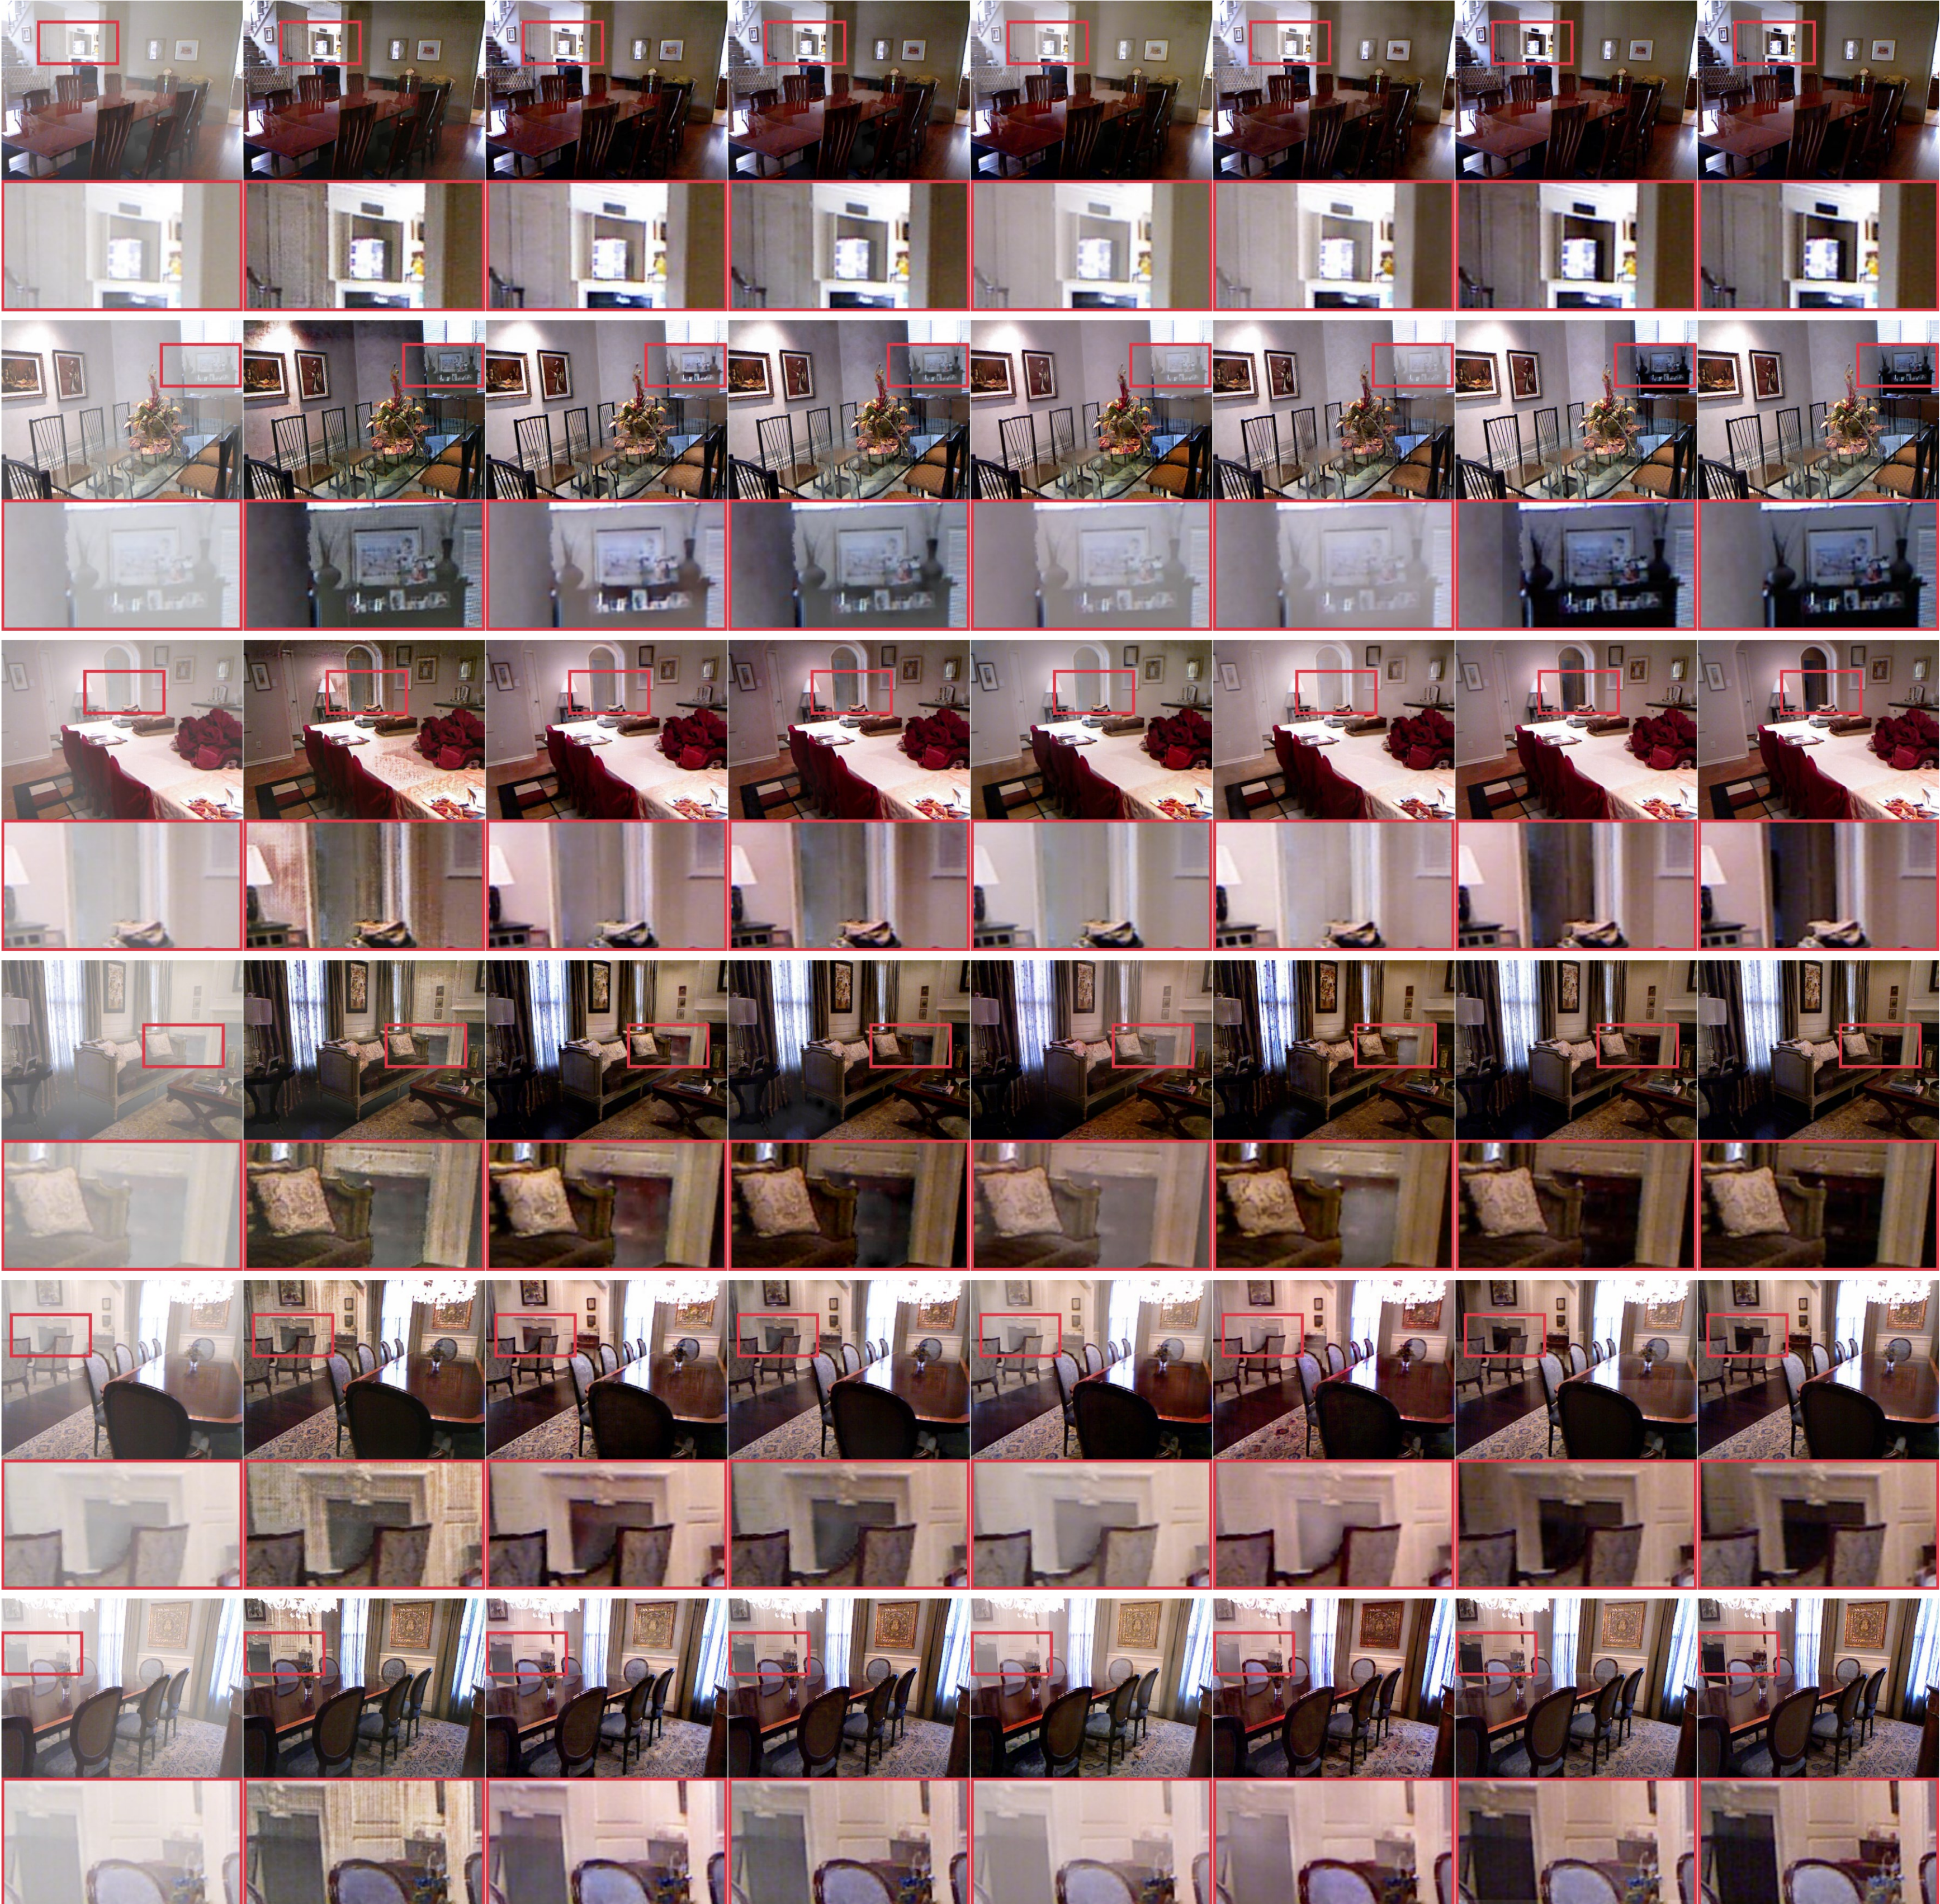

Hazy

RefinedNet

CDD-GAN

D4

UCL-Dehaze

ODCR

Ours

GT



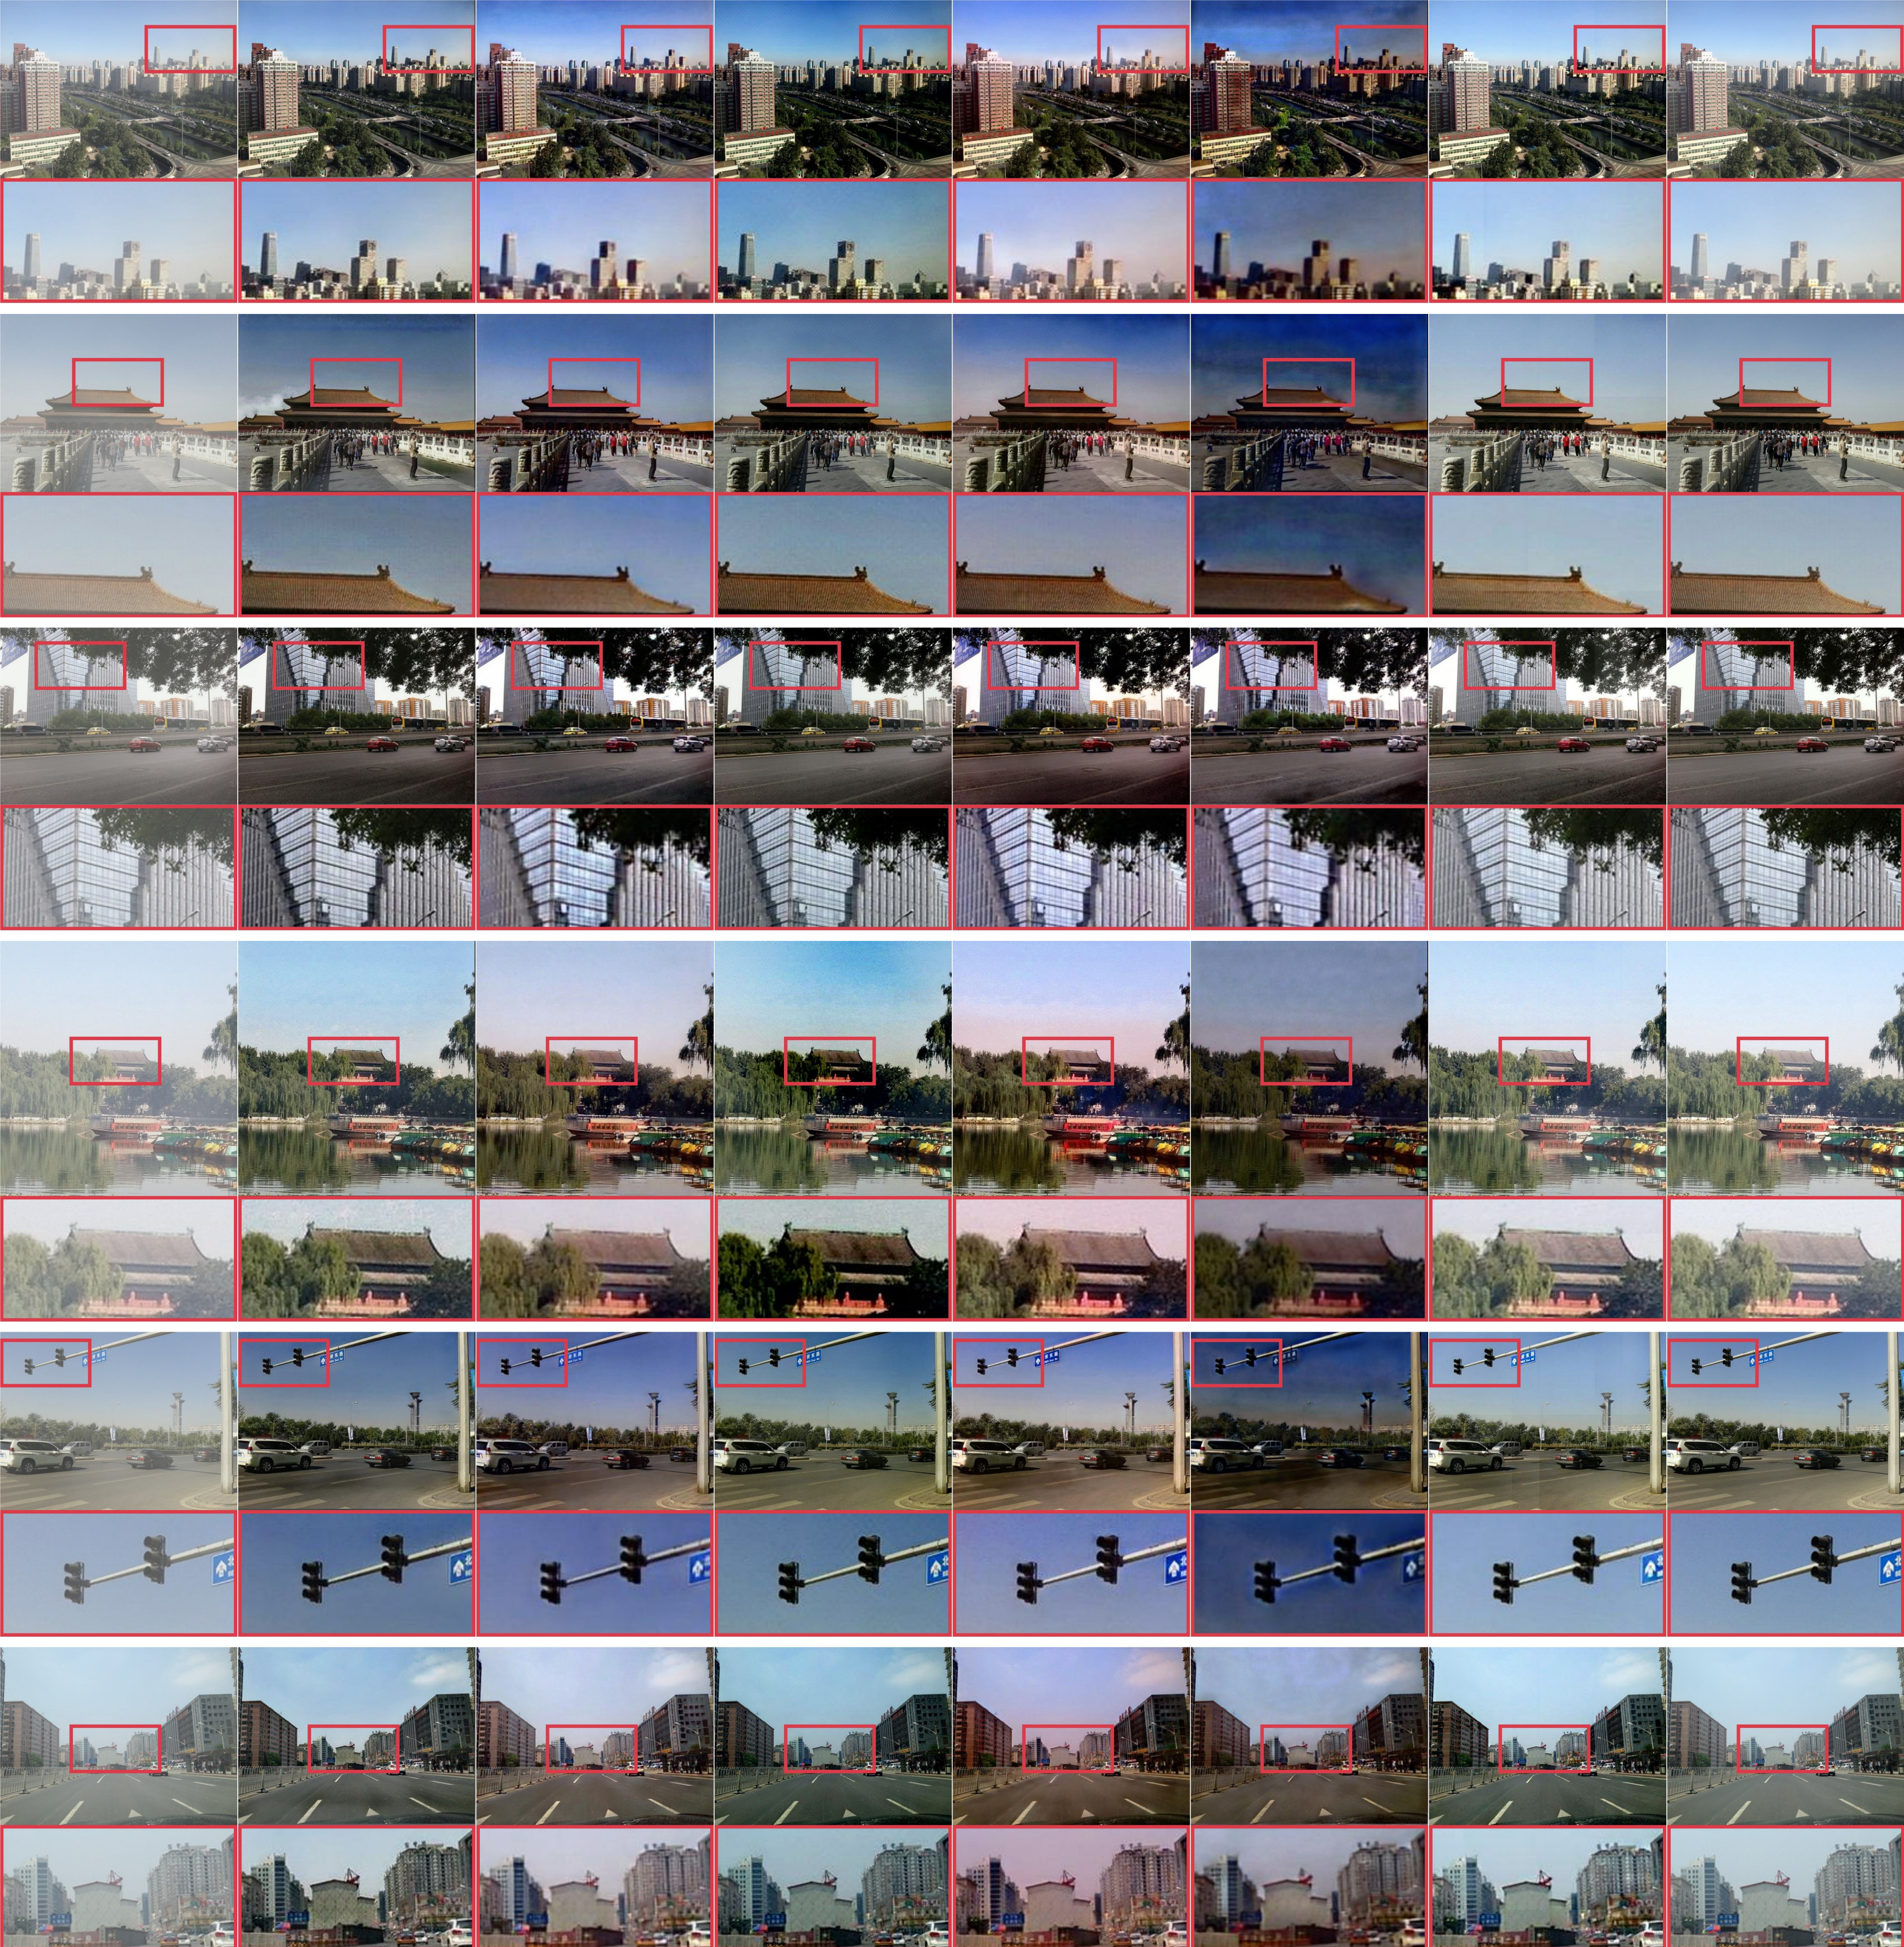

Hazy

RefinedNet

CDD-GAN

D4

UCL-Dehaze

ODCR

Ours

GT



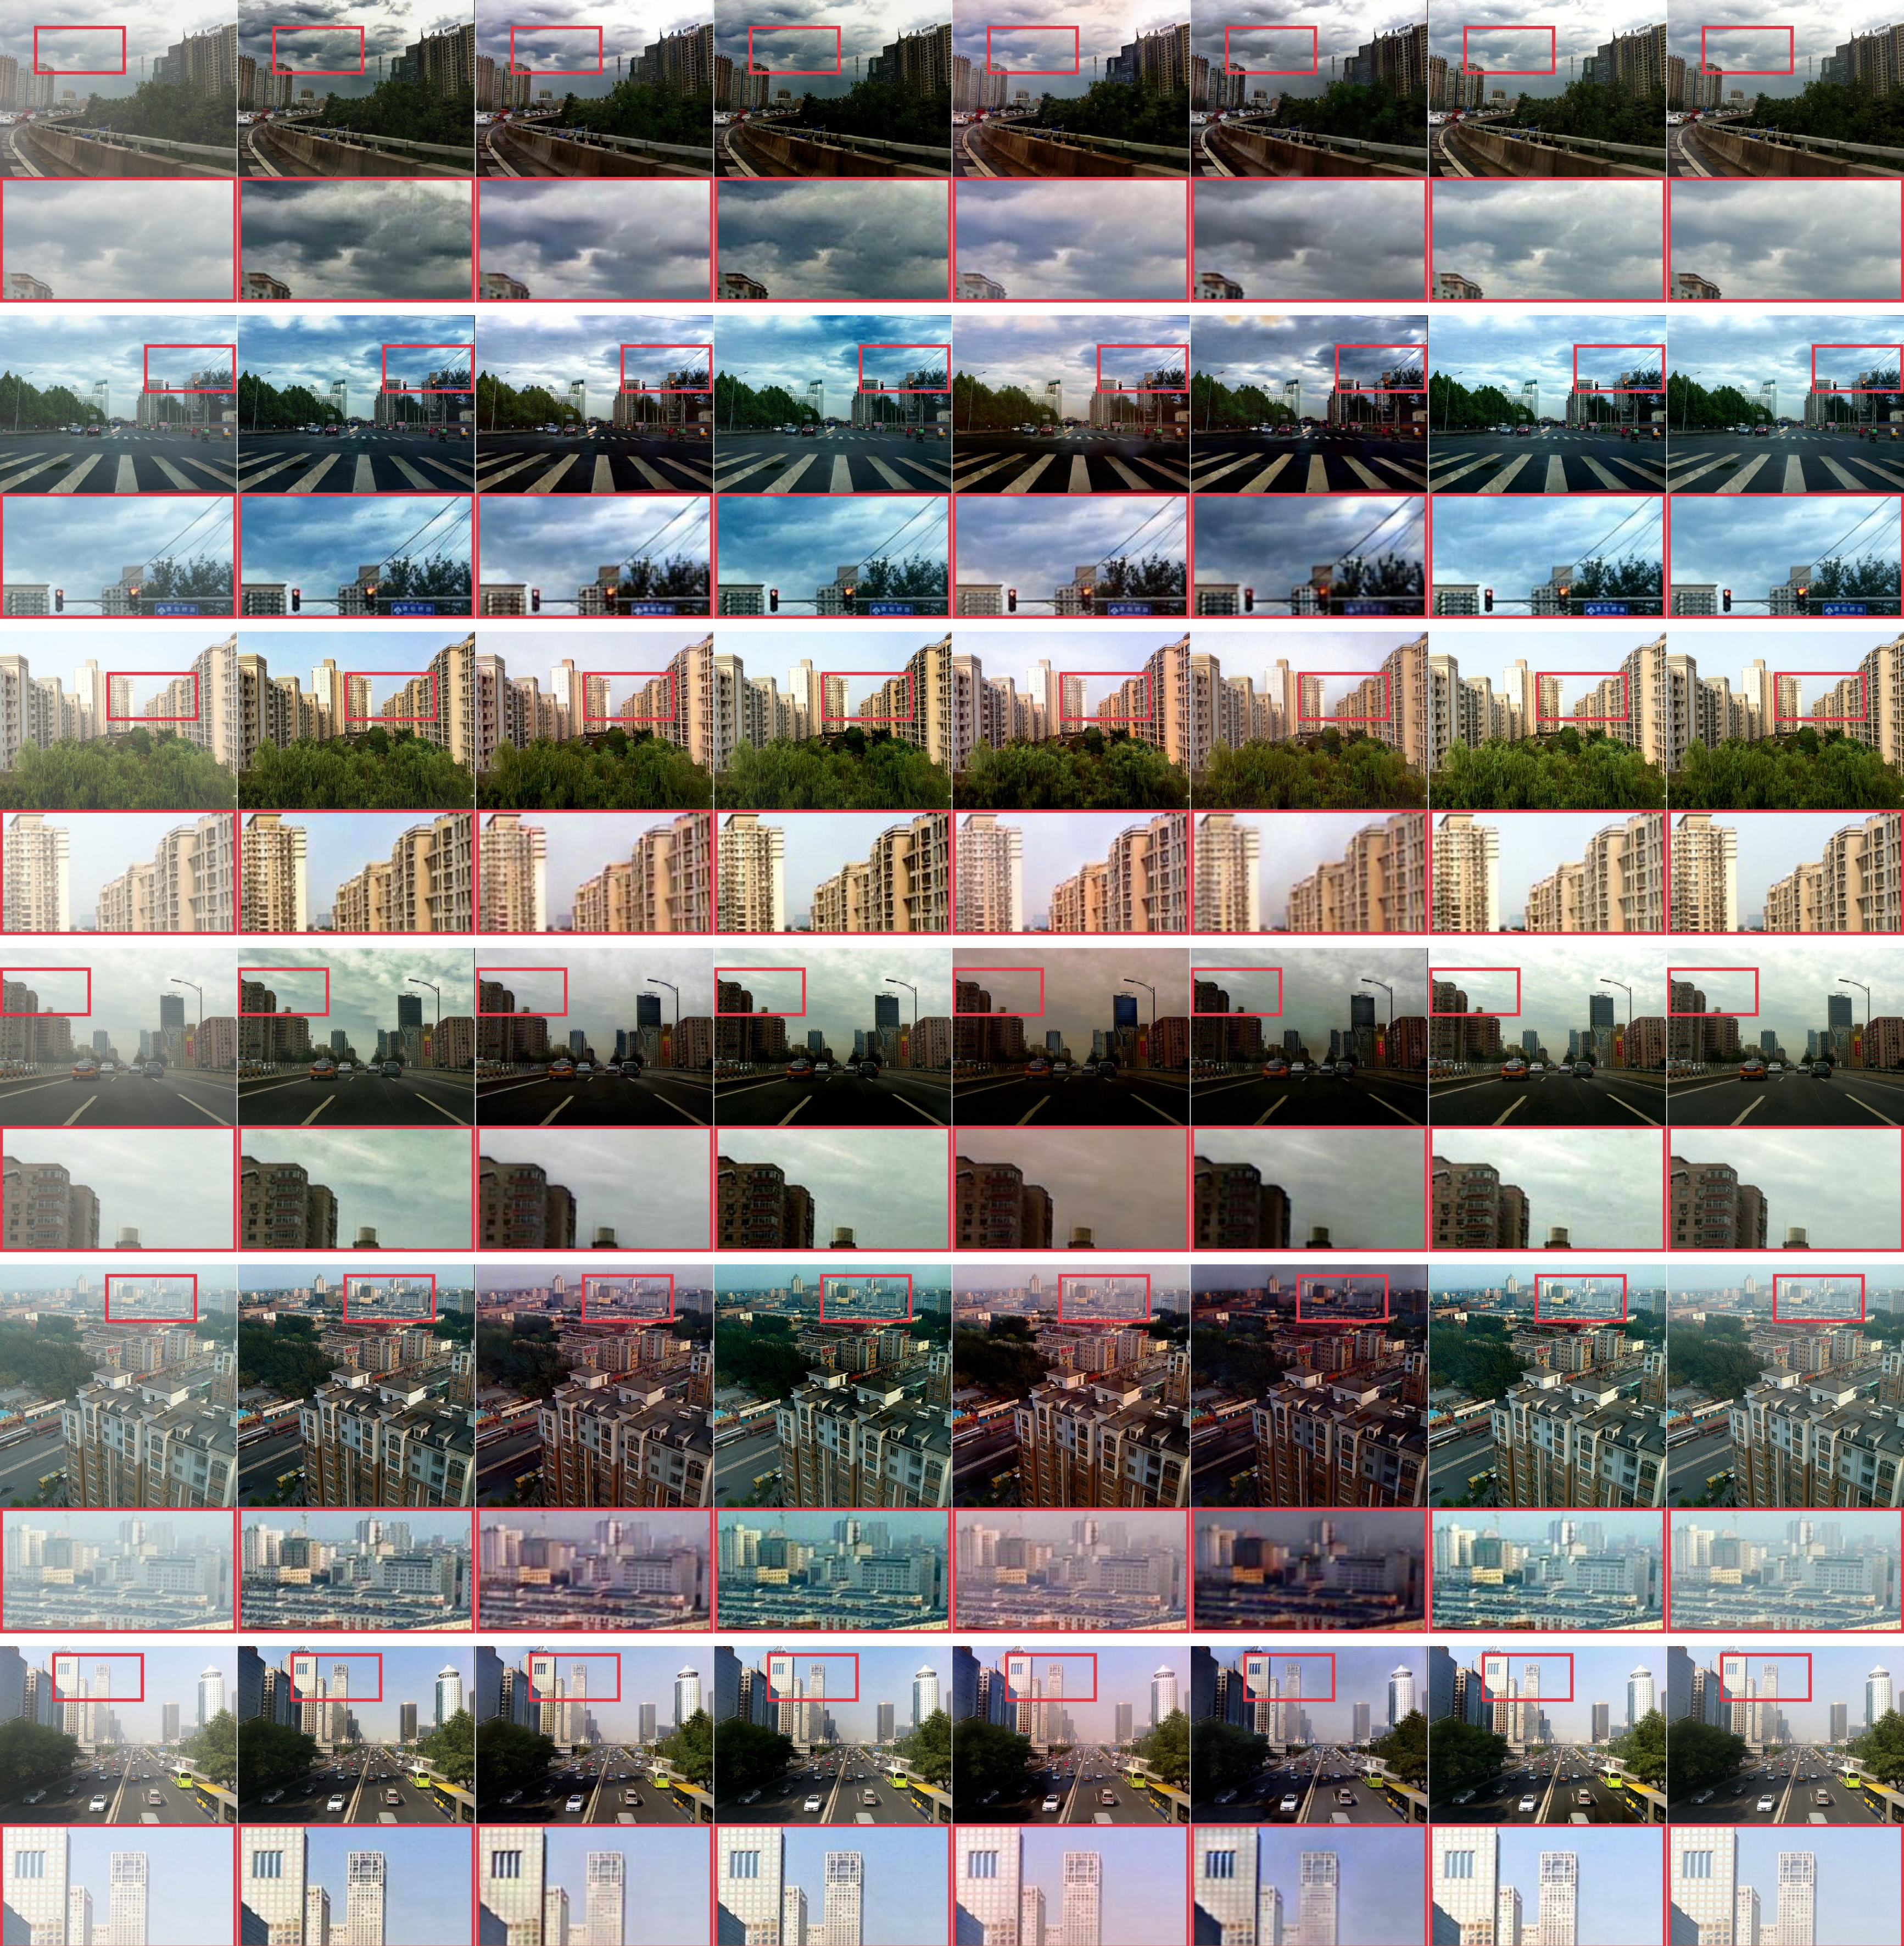

Hazy

RefinedNet

CDD-GAN

D4

UCL-Dehaze

ODCR

Ours

GT



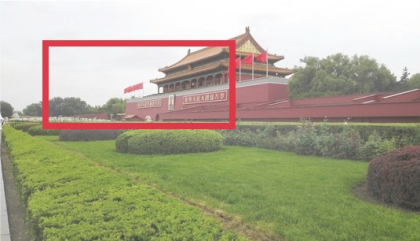

Hazy

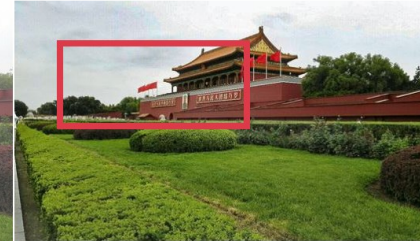

RefineDNet

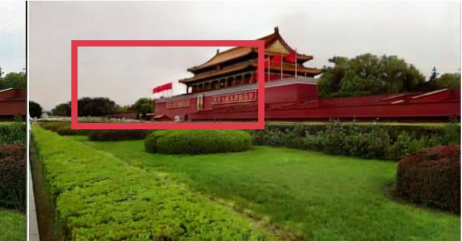

CDD-GAN

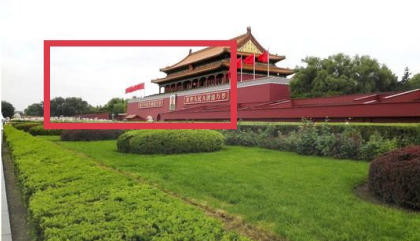

D4

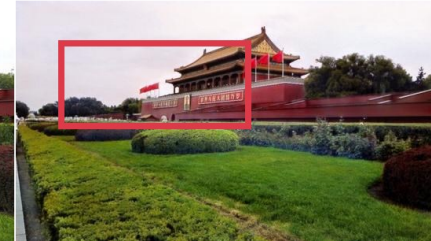

UCL-Dehaze

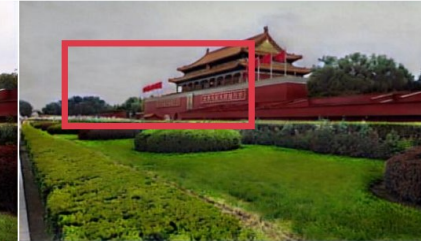

ODCR

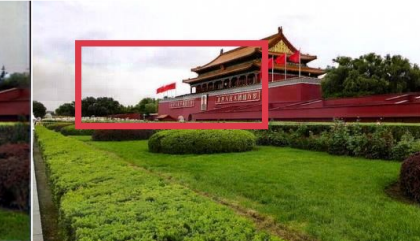

Ours

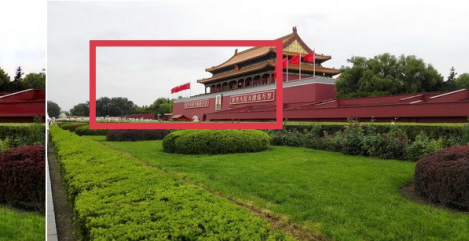

GT



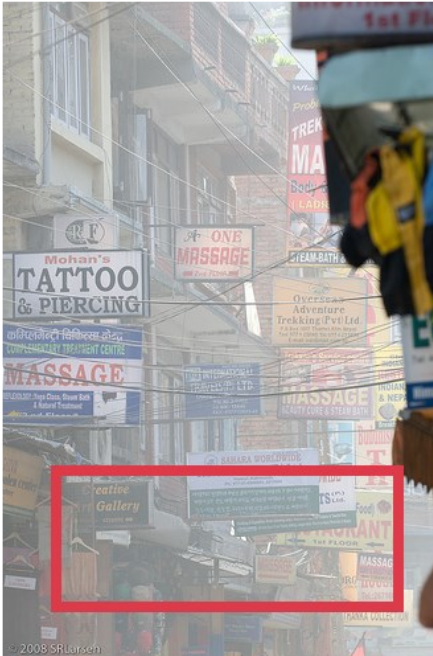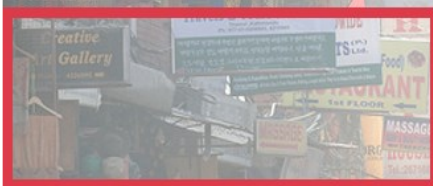

Hazy

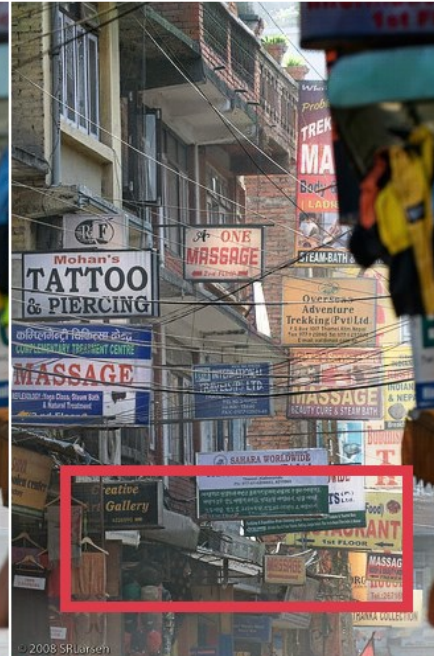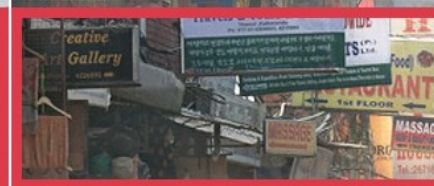

RefineDNet

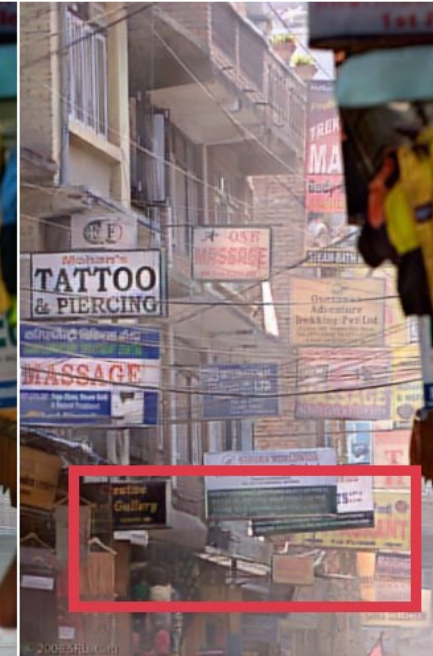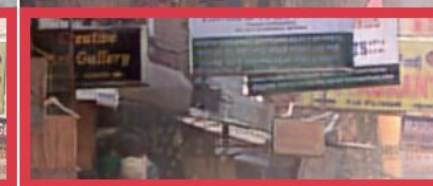

CDD-GAN

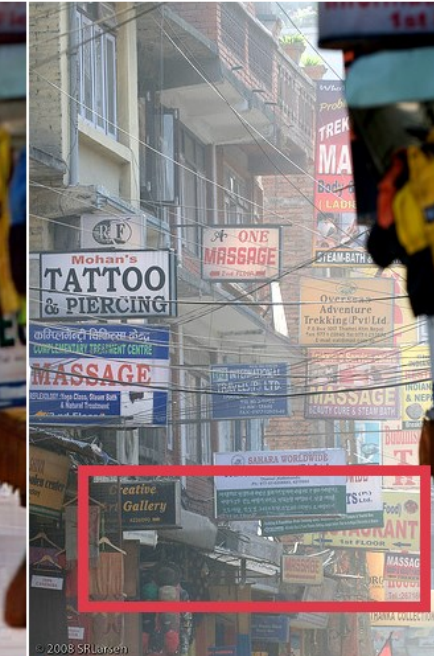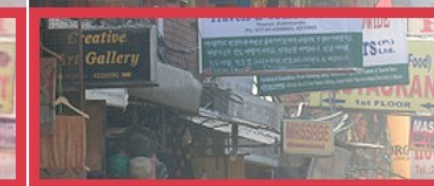

D4

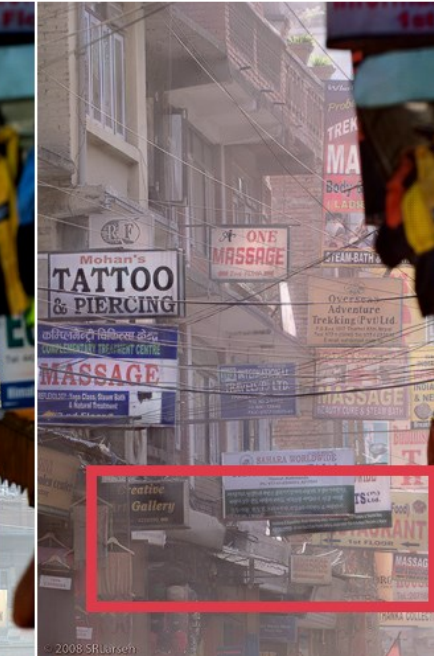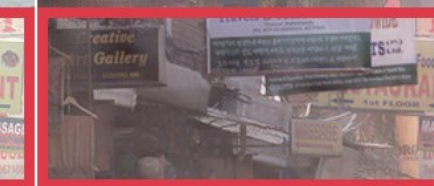

UCL-Dehaze

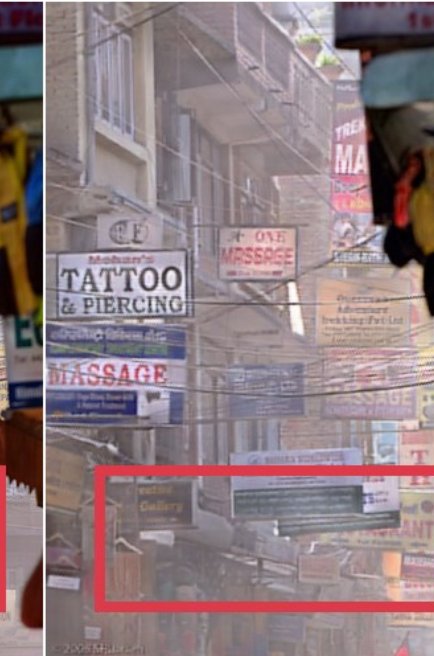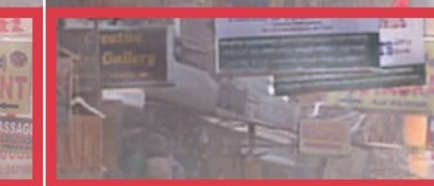

ODCR

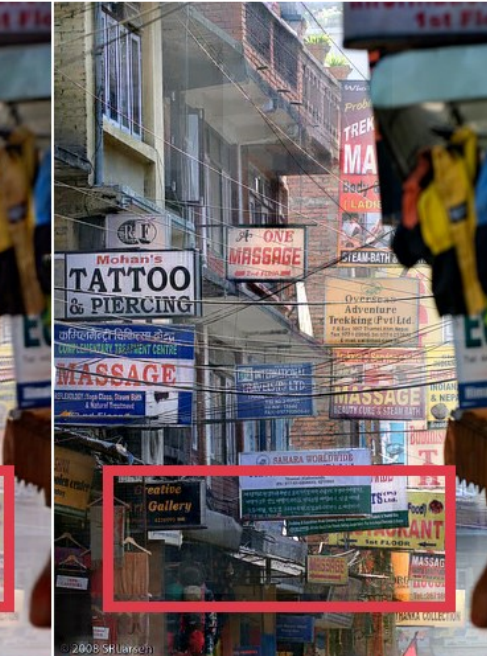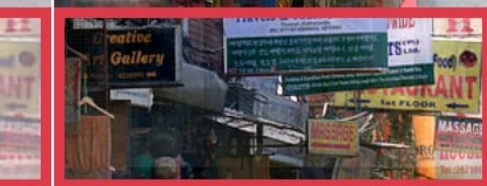

Ours



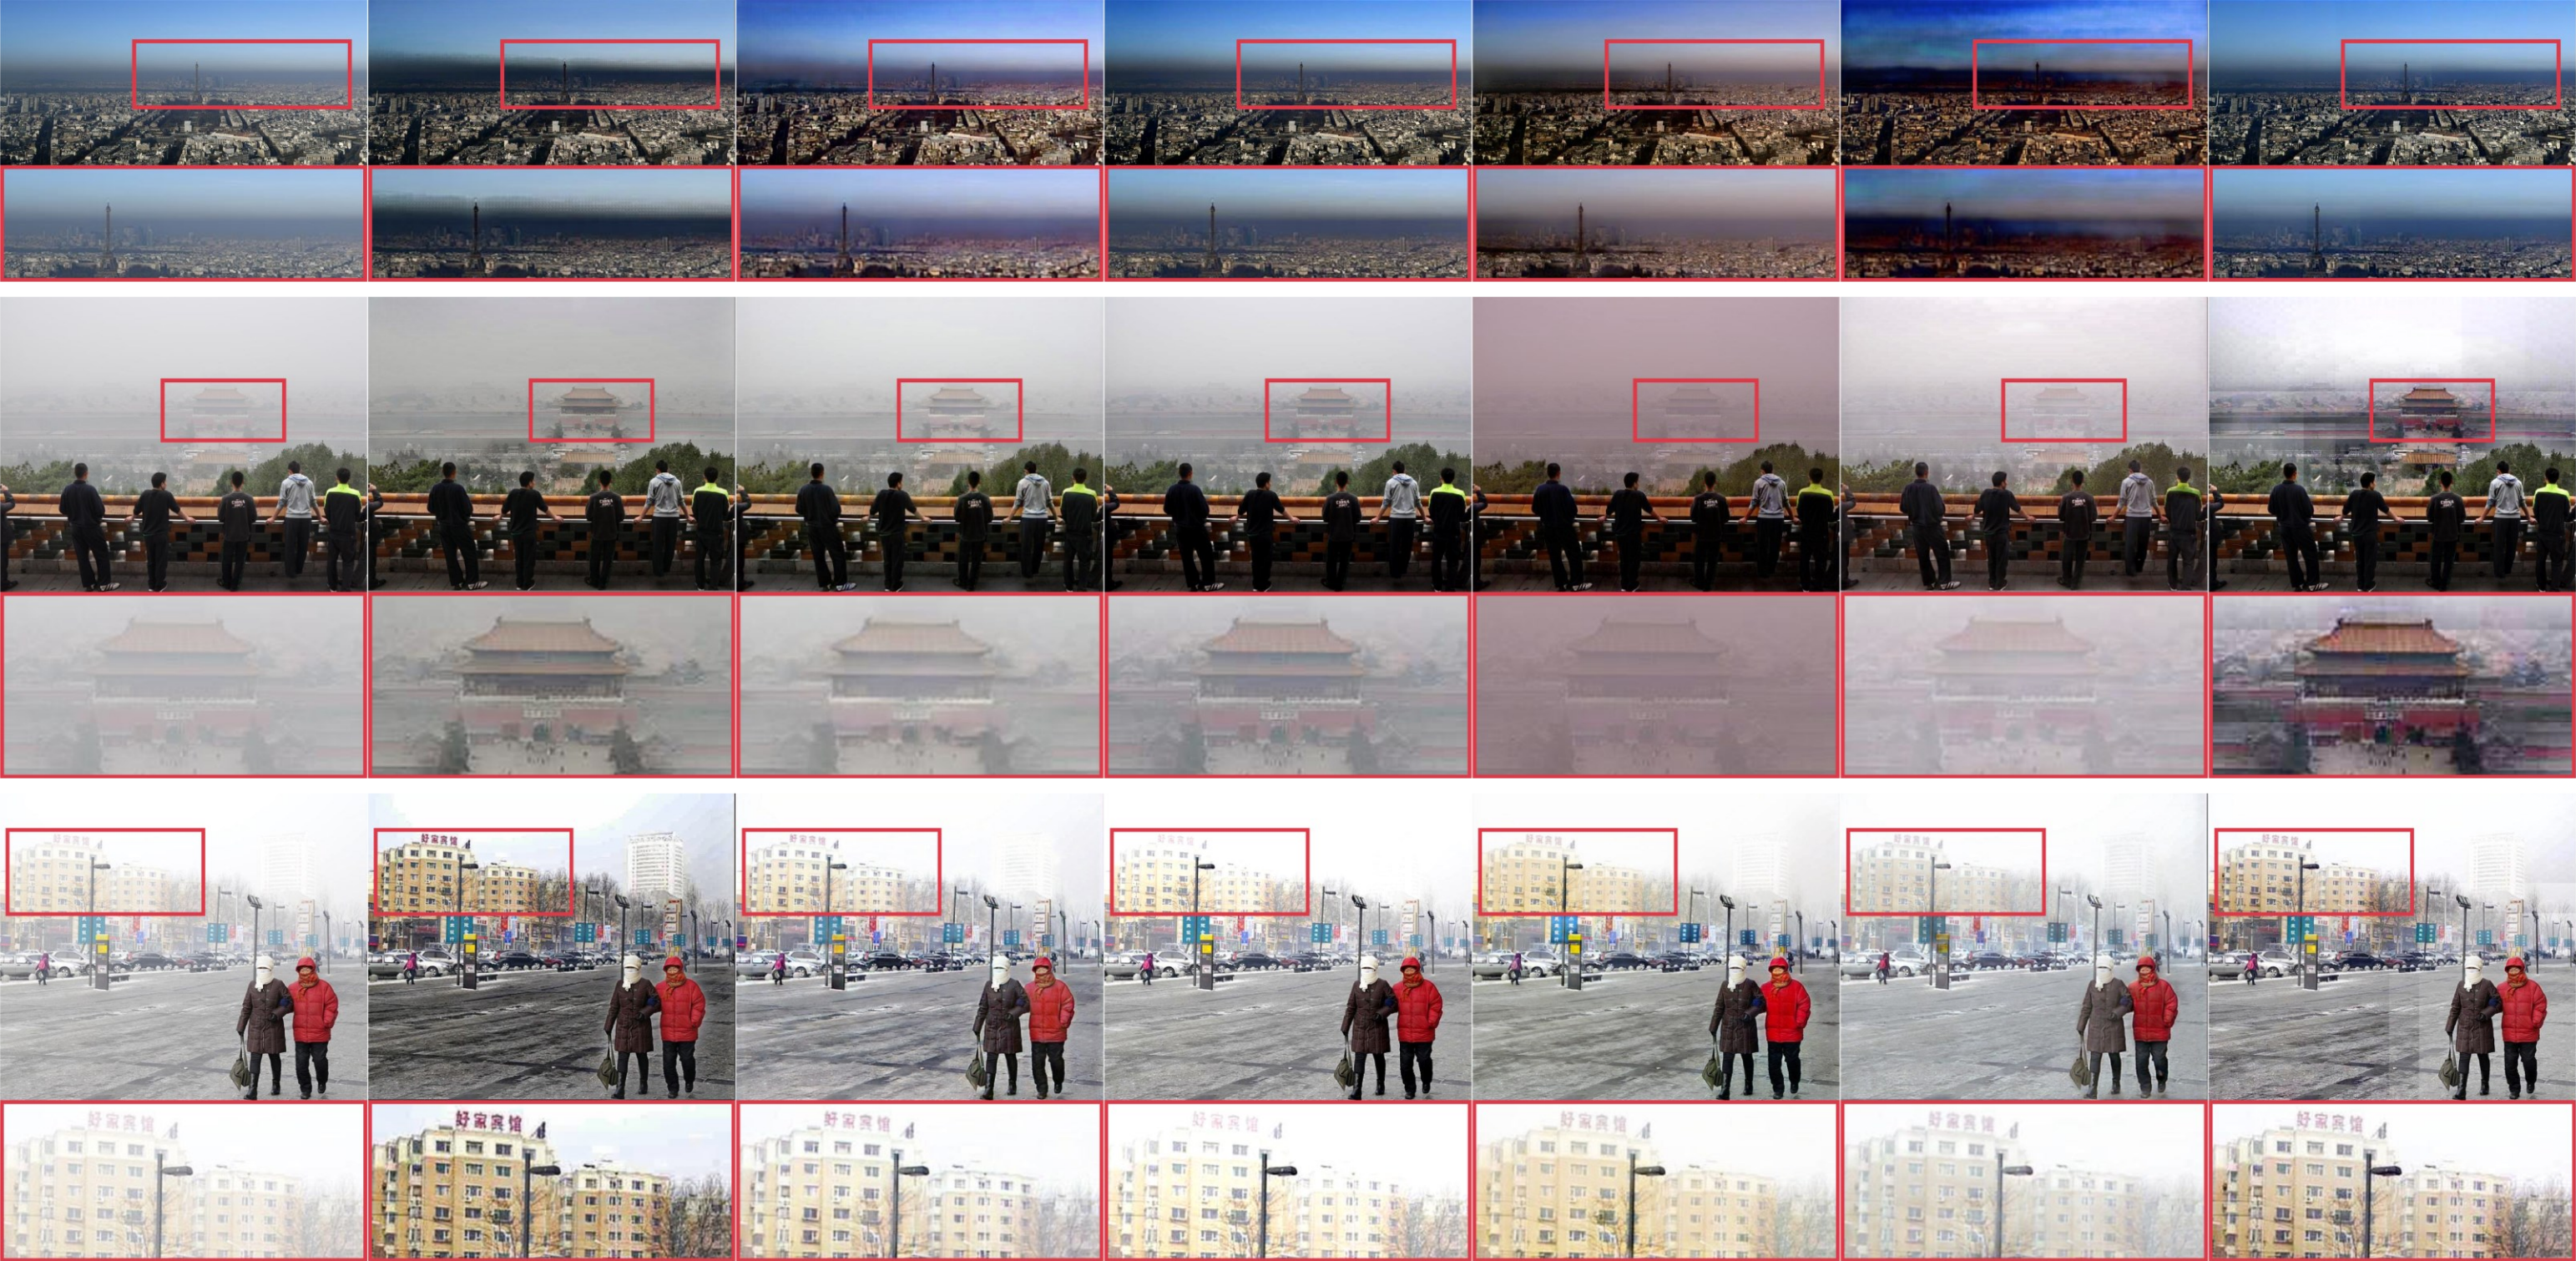

Hazy

RefineDNet

CDD-GAN

D4

UCL-Dehaze

ODCR

Ours
